# Supplementary material for: Search for the Standard Model Higgs boson produced in association with a vector boson and decaying to a b-quark pair with the ATLAS detector
Source: arXiv:1207.0210 source file (2012-11-19)
Supplement: Supplementary file 1 [file appendix.tex]

\section{Additional Material}

This appendix contains additional material to be approved for public
presentations. They are also included in the support notes for this
paper: ATL-COM-PHYS-2011-1648 and ATL-COM-PHYS-2012-062, which can be
found in the CERN Document Server records
\verb+https://cdsweb.cern.ch/record/1404176+ and
\verb+https://cdsweb.cern.ch/record/1418230+.

\begin{figure}[htb]
  \begin{center}
    \includegraphics[width=0.49\textwidth]{figaux_06.eps}
    \caption
	{The distribution of the number of $b$-tagged jets in events
containing at least two reconstructed jets for the \zhtollbb
selection.}
	\label{fig:A6}
  \end{center}
\end{figure}

\begin{figure}[htb]
  \begin{center}
    \includegraphics[width=0.49\textwidth]{figaux_07.eps}
    \caption
	{ Control region for the \zhtollbb analysis: invariant mass
formed from the two highest \pT\ jets where only one jet is
$b$-tagged.  }
	\label{fig:A7}
  \end{center}
\end{figure}

\begin{figure}[htb]
  \begin{center}
    \includegraphics[width=0.49\textwidth]{figaux_08.eps}
    \caption
	{ The invariant mass formed from two $b$-tagged jets, using
the sidebands of the $m_{\ell\ell}$ distribution, for the $ZH$
analysis and the selection for events with \met\ $>50$~\gev. The Monte
Carlo distribution is shown after applying the $Z+jets$ and top
normalization corrections derived in the fit.  }
	\label{fig:A8}
  \end{center}
\end{figure}

\begin{figure}[htb]
  \begin{center}
    \includegraphics[width=0.49\textwidth]{figaux_09.eps}
    \caption
	{ The distribution of the number of $b$-tagged jets in events
	 containing exactly two jets for the \whtolnubb selection.  }
	\label{fig:A9}
  \end{center}
\end{figure}

\begin{figure}[htb]
  \begin{center}
    \includegraphics[width=0.49\textwidth]{figaux_10a.eps}
    \includegraphics[width=0.49\textwidth]{figaux_10b.eps}
    \caption
	{ The $b$-tagging weight for both jets without applying the
	  $b$-tagging cut for the \zhtollbb\ analysis (top) and the $WH$
	  analysis (bottom).  The data are shown as points with error
	  bars.  The contributions of $V$+$c$, $V$+$b$ and $V$+$l$ and
	  the background processes are shown.  The full line shows the
	  result of the fit with the normalization of the $c$ and $l$
	  MC templates treated as free parameters.
	}
	\label{fig:A11}
  \end{center}
\end{figure}

\begin{figure}[htb]
  \begin{center}
    \includegraphics[width=0.49\textwidth]{figaux_11a.eps}
    \includegraphics[width=0.49\textwidth]{figaux_11b.eps}
    \caption
	{ The comparison of the data \ptZ\ distribution in the $ZH$
	  analysis with the {\sc SHERPA} $Z$+jets MC plus background
	  in the \mbb\ sidebands for two tagged jets (top).  The
	  dashed lines show the systematic uncertainty due to the
	  reweight of \ptZ\ . The data are also compared with the {\sc
	  ALPGEN} $Z$+jets MC plus background. The bottom plot is the
	  same but the data and models are divided by the expectation
	  from the {\sc SHERPA} $Z$+jets MC.
	}
	\label{fig:A12}
  \end{center}
\end{figure}

\begin{figure}[htb]
  \begin{center}
    \includegraphics[width=0.49\textwidth]{figaux_12.eps}
    \caption
	{ The di-$b$-jet invariant mass for the control region for
top-quark events in the \whtolnubb analysis where the requirement on
the number of jets is changed from two to three.  }
	\label{fig:A10}
  \end{center}
\end{figure}

\begin{figure}[htb]
  \begin{center}
    \includegraphics[width=0.49\textwidth]{figaux_13.eps}
    \caption{\label{fig:app:trig_eff_xe70_Wmunu_data}
      The trigger efficiency of {\tt EF\_xe70\_noMu} as function of \met,
      measured from the data and MC for the $W(\rightarrow\mu\nu)+$jets process.
    }
    \label{fig:app:dijetmassSBComp}
  \end{center}
\end{figure}

\begin{figure}[htb]
  \begin{center}
    \includegraphics[width=0.49\textwidth]{figaux_14.eps}
    \caption
	{\zhtollbb candidate event. }
	\label{fig:app:eventDisplayZHllbb}
  \end{center}
\end{figure}

\begin{figure}[htb]
  \begin{center}
    \includegraphics[width=0.49\textwidth]{figaux_15.eps}
    \caption
	{\whtolnubb candidate event. }
	\label{fig:app:eventDisplayWHlvbb}
  \end{center}
\end{figure}

\begin{figure}[htb]
  \begin{center}
    \includegraphics[width=0.49\textwidth]{figaux_16.eps}
    \caption
	{\zhtovvbb candidate event. }
	\label{fig:app:eventDisplayZHvvbb}
  \end{center}
\end{figure}
